# Supplementary material for: Search for heavy resonances decaying to a $Z$ boson and a photon in $pp$ collisions at $\sqrt{s}=13$ TeV with the ATLAS detector
Source: arXiv:1607.06363 source file (2016-11-30)
Supplement: Supplementary file 1 [file appendix.tex]

\onecolumn
\section*{Auxiliary material}
\subsection*{Signal distributions}

\begin{figure}[!htbp]
  \begin{center}
    \includegraphics[width=0.6\columnwidth]{figures/sigjet_conf}
    \caption{Comparison of calibrated large-$R$ jet mass distributions for the MC $gg\to X \to Z \gamma \to q\bar{q}\gamma$ signal events, generated for three different $m_X$ hypotheses: $m_X=750$~\GeV\ (black points), $m_X=1500$~\GeV\ (red squares), $m_X=2500$~\GeV\ (green triangles). Events passing the photon and jet kinematic analysis selection criteria are used.}    
    \label{fig:jetmass}
  \end{center}
\end{figure}

\begin{figure}[!htbp]
  \begin{center}
    \includegraphics[width=0.6\columnwidth]{figures/dRll}
    \caption{$\Delta R$ separation at generator-level
      between the two leptons from the decays of the $Z$ bosons 
      from $X\to Z\gamma$ in signal samples of with mass $m_X$
      between 200~\GeV\ and 2~\TeV.}
    \label{fig:dRll}
  \end{center}
\end{figure}

\begin{figure}[!htbp]
  \begin{center}
    \subfigure[]{\includegraphics[width=0.6\columnwidth]{figures/genphpt}}
    \subfigure[]{\includegraphics[width=0.6\columnwidth]{figures/genphptovermllg}}
        \caption{Generator-level distributions of the photon
          transverse momentum before (a) or after (b)
          dividing it by the three-body mass $m_{\ell\ell\gamma}$,
          in $X\to Z\gamma$ decays.}
    \label{fig:phpt}
  \end{center}
\end{figure}

\clearpage

\subsection*{Signal efficiency}

\begin{figure}[!htbp]
  \begin{center}
    \includegraphics[width=0.6\columnwidth]{figures/efficiency_with_BR}
    \caption{Efficiency as a function of the resonance mass $m_X$
      of the lepton selection (filled circles)
      and of the hadronic selection (open squares), for simulated $X\to Z\gamma$ events
      in which the $Z$ bosons decay inclusively.
      The solid and dashed lines represent an interpolation
      with a smooth function (of the type $a+be^{cm_X}$) and a linear, piece-wise
      interpolation of the efficiencies of the leptonic and hadronic selections,
      respectively.}
    \label{fig:efficiency_with_BR}
  \end{center}
\end{figure}

\clearpage

\subsection*{Data-MC comparisons}

\begin{figure}[!htbp]
  \begin{center}
    \includegraphics[width=0.6\columnwidth]{figures/jetmass_conf}
    \caption{Calibrated large-$R$ jet mass distribution for data events (black points) and MC $gg\to X \to Z \gamma \to q\bar{q}\gamma$ signal events with $m_X=750~\GeV$ (red histogram), passing the photon and jet kinematic analysis selection criteria. The jet substructure requirements are not applied. The MC signal yield is normalized to the data for illustration purpose.}
    \label{fig:jetmass2}
  \end{center}
\end{figure}

\begin{figure}[!htbp]
  \begin{center}
    \includegraphics[width=0.6\columnwidth]{figures/mjfull_conf}
    \caption{$m_{J\gamma}$ distribution in data for events passing the analysis selection criteria. The region used for the final fit ($m_{J\gamma}>640$~\GeV) is indicated by the blue vertical line.}
    \label{fig:mJgamma_datamc}
  \end{center}
\end{figure}

\clearpage

\subsection*{Additional limit plots and p0 plot}

\begin{figure}[!htbp]
\centering
\subfigure[]{\includegraphics[width=0.48\columnwidth]{figures/limit_leptonic_log}}
\subfigure[]{\includegraphics[width=0.48\columnwidth]{figures/limit_hadronic_log}}
    \caption{Observed (solid line) and median expected (dashed line)
      95\% CL upper limits on the product of the production cross section times
      the branching ratio for the decay to a $Z$ boson and a photon
      of a narrow scalar boson $X$.
      The limits are set as a function
      of the boson mass $m_X$, using either $Z$ bosons reconstructed
      in decays to electrons and muons (a) or hadrons (b).
      The green and yellow bands correspond to the $\pm 1\sigma$ and
      $\pm 2\sigma$ intervals for the expected upper limit,
      respectively.}
     \label{fig:limit_data_logscale}
 \end{figure}

\begin{figure}[!htbp]
  \centering
  \includegraphics[width=0.8\columnwidth]{limit_both_log}
  \caption{Observed (solid lines) and median expected (dashed lines)
    95\% CL limits on the product of the production cross section times
    the branching ratio for the decay to a $Z$ boson and a photon
    of a narrow scalar boson $X$, as a function of the boson mass $m_X$.
    The black lines correspond to the limits set with the $J\gamma$ final
    state, the blue lines correspond to the limits set with the
    $\ell\ell\gamma$ final state.
    The dark green and dark yellow hatched bands correspond to the
    $\pm 1\sigma$ and
    $\pm 2\sigma$ intervals for the expected upper limit,
    respectively, set with the $J\gamma$ final state.
    The green and yellow solid bands correspond to the $\pm 1\sigma$ and
    $\pm 2\sigma$ intervals for the expected upper limit,
    respectively, set with the $\ell\ell\gamma$ final state.
  }
  \label{fig:limit_data_both}
\end{figure}

\begin{figure}[!htbp]
\centering
\subfigure[]{\includegraphics[width=0.48\columnwidth]{p0_leptonic_uncapped}}
\subfigure[]{\includegraphics[width=0.48\columnwidth]{p0_hadronic_uncapped}}
    \caption{Observed $p_0$ (compatibility of
       the data with the background-only hypothesis) as a function
       of the mass of a narrow scalar boson decaying to $Z\gamma$,
       using $Z$ bosons reconstructed in decays to electrons
       and muons (a) or hadrons (b).}
     \label{fig:p0_data}
 \end{figure}

\clearpage

\subsection*{Event displays}

\begin{figure}[!htbp]
  \centering
  \includegraphics[width=0.7\columnwidth,angle=270]{figures/event_display281411Det}
  \caption{Event display of the highest invariant mass $\mu\mu\gamma$ candidate passing the event selection. The transverse momenta of the photon (in green) and of the two muons (in red) are 491, 488, and 48~\GeV, respectively. The dimuon invariant mass is 93.9~\GeV\ and the $\mu\mu\gamma$ invariant mass is 1030~\GeV.
    Only inner-detector tracks with $\pT>1$~\GeV\ and calorimeter cells with energy deposits larger than 250~\MeV\ are shown.}
  \label{fig:evt_display_mumugamma_threedim}
\end{figure}

\begin{figure}[!htbp]
  \centering
  \includegraphics[width=0.7\columnwidth]{figures/JiveXML_283429_1488985140-YX-RZ-LegoPlot-EventInfo-2016-03-09-14-06-52}
  \caption{Event display of the highest-invariant mass $ee\gamma$ candidate passing the event selection. The transverse momenta of the photon (green bar) and of the two electrons (blue bars) are 795, 528, and 135~\GeV, respectively. The dielectron invariant mass is
    91.7~\GeV\ and the $ee\gamma$ invariant mass is 1470~\GeV.
    Only inner-detector tracks with $\pT>5$~\GeV\ and calorimeter cells with energy deposits larger than 250~\MeV\ are shown.}
    \label{fig:evt_display_eegamma}
\end{figure}

\begin{figure}[!htbp]
\centering
    \includegraphics[width=0.7\columnwidth]{figures/JiveXML_283429_1488985140-RZ-LegoPlot-EventInfo-2016-03-09-14-07-28}
    \caption{Event display of the highest-invariant mass $ee\gamma$ candidate passing the event selection (lateral view). The transverse momenta of the photon and of the two electrons are 795, 528, and 135~\GeV, respectively. The dielectron invariant mass is
      91.7~\GeV\ and the $ee\gamma$ invariant mass is 1470~\GeV.
      Only inner-detector tracks with $\pT>5$~\GeV\ and calorimeter cells with energy deposits larger than 250~\MeV\ are shown.}
    \label{fig:evt_display_eegamma_lateralview}
\end{figure}
